# Supplementary material for: Raw Image Reconstruction with Learned Compact Metadata
Source: arXiv:2302.12995 source file (2023-02-28)
Supplement: Supplementary file 1 [file appendix.tex]

\textit{In the supplementary material, we provide more details about the implementation details, including the network design, and the details of the visualization in the main paper. Besides, we provide more ablation studies and qualitative comparison, including the reconstruction qualities under different bpp and the effectiveness of learned sampling masks, to demonstrate the effectiveness of the proposed method.}
\section{Implementation details}
\textbf{Hyper-parameter $\lambda$ in Eq. 3.}
For the hyper-parameter $\lambda$ which controls the tradeoff between the codelength and reconstruction quality defined in Eq. 3 in the main paper, we set it to $1$ for uncompressed sRGB images and $0.05$ for the compressed ones. We use a higher $\lambda$ for the uncompressed sRGB images because it is relatively easier to do the reconstruction with high fidelity using a small codelength based on the uncompressed images.

\textbf{Model architecture in Fig. 3.}
We further introduce details of the proposed architecture as a supplement to Fig. 3 and Fig. 4 in the main paper. For the residual connection with a different channel number in Fig. 3 of the main paper, we use an $1\times1$ convolutional kernel in the residual connection to make them compatible. We adopt the same attention block in \cite{cheng2020learned}. In addition, $/2$ in $h_a$ in Fig. 2 of the main paper represents the downsampling operation, \textit{i.e.}, the resolution of auxiliary variable $v$ is down-sampled by a factor of 4.
% \section{Architecture Details}

\textbf{Quantization error map in Fig. 2.}
To illustrate the information loss caused by the non-linear transform and quantization step is non-uniform, we display the quantization error map in the main paper in Fig. 2. The quantization error map is estimated as follows:
For a raw image $\mathbf{x}$, we first obtain its rendered sRGB image $\mathbf{y}$ without quantization. 
We calculate and save the mapping relationship $\mathbf{w}=\mathbf{x}/(\mathbf{y}+\epsilon)$ where $/$ is a pixel-wised division and $\epsilon$ is a small constant, \textit{i.e.}, 1e-3.
For an sRGB image after quantization $\hat{\mathbf{y}}$, the quantization error map $\mathbf{e}$ is calculated as $\mathbf{e} = |\mathbf{w} \cdot (\mathbf{\hat{y}}+\epsilon) - \mathbf{x}|$.

\textbf{The estimation of bpp maps in Fig. 9.} We estimate the likelihood of latent code $y$ and $z$ using Eq. 4 in the main paper. The number of bits can be estimated by $-\log_2 p(x)$ where $p(x)$ is the estimated likelihood. 
Specifically, since the spatial resolution of $\mathbf{v}$ is smaller than $\mathbf{z}$, we interpolate the estimated bpp maps of $\mathbf{v}$ to the same size as $\mathbf{z}$ and keeps the total bits of $\mathbf{v}$ unchanged. Finally, the visualization of the bits map in Fig. 9 includes bits both allocated by $\mathbf{z}$ and $\mathbf{v}$.

\begin{figure*}
    \centering
    \begin{subfigure}{0.33\linewidth}
    {
    \includegraphics[width=1\linewidth]{figure/appendix/PSNR_Samsung.pdf}
    \includegraphics[width=1\linewidth]{figure/appendix/SSIM_Samsung.pdf}
    }
    \caption{Samsung NX2000}
    \label{fig:pixelcnn}
    \end{subfigure}
    \begin{subfigure}{0.33\linewidth}
    {
    \includegraphics[width=1\linewidth]{figure/appendix/PSNR_Olympus.pdf}
    \includegraphics[width=1\linewidth]{figure/appendix/SSIM_Samsung.pdf}
    }
    \caption{Olympus E-PL6}
    \label{fig:pixelcnn}
    \end{subfigure}
    \begin{subfigure}{0.33\linewidth}
    {
    \includegraphics[width=1\linewidth]{figure/appendix/PSNR_Sony.pdf}
    \includegraphics[width=1\linewidth]{figure/appendix/SSIM_Samsung.pdf}
    }
    \caption{Sony SLT-A57}
    \label{fig:pixelcnn}
    \end{subfigure}

    \hfill
    \caption{The reconstruction qualities of models under different bpp. We evaluate the performance of models using compressed JPEG images with a quality factor of $10$ from the NUS dataset~\cite{cheng2014illuminant}. The file size of JPEG images is also taken into consideration for the calculation of the bpp, \textit{e.g.}, the bpp of InvISP is equal to the bpp of JPEG images since InvISP does not save additional metadata.}
    \label{fig:bpp}
\end{figure*}

\section{Additional results}

\subsection{Computational cost}
Our method can be trained and evaluated on a single RTX A5000 GPU. Specifically, we evaluate the computational cost of our proposed method and other SOTA methods. The results are shown in Table \ref{tab:cost} measured by a commonly used library \textit{thop}~\footnote{\url{https://github.com/Lyken17/pytorch-OpCounter}}.
As we can see in the table, with the help of our proposed sRGB-guided context model, the context model becomes feasible in the raw image reconstruction task where the feature resolution is much higher. Compared with other learning based models, our method is lightweight with fewer parameters. In addition, we achieve comparable speed with other DNN-based networks, \textit{e.g.}, InvISP~\cite{xing2021invertible} and SAM~\cite{punnappurath2021spatially}, and faster speed than test-time model SAM~\cite{punnappurath2021spatially}.
Besides, the speed bottleneck of our proposed method becomes the arithmetic coding instead of the previous context model~\cite{minnen2018joint, cheng2020learned}.
Our proposed method can be further accelerated by running the arithmetic coding on GPUs \cite{gpuar, chen2011accelerating, vsupol2005arithmetic}, which is out of the scope of the paper.

\begin{table}[htbp]
    \centering
    \begin{tabular}{ccccc}
    \toprule
         & Parameters & FLOPs & Compress \& Decompress time\\
    \midrule
        InvISP~\cite{xing2021invertible} & 1.41MB & 18.06T & 5.13s\\
        SAM~\cite{punnappurath2021spatially} (bpp 9.56e-4) & N/A & -- & 16.40s\\
        SAM~\cite{punnappurath2021spatially} (bpp 9.52e-3) & N/A & -- & 103.92s\\
        Nam~\textit{et al.}\cite{nam2022learning} & 2.59MB & 5.23T & 1.50s\\
        Ours (serial) & 0.53MB & -- & $>$ 10 hours\\
        \rowcolor[HTML]{EFEFEF} Ours & 0.55MB & 5.82T & 1.60+6.72 (arithmetic coding on CPU)=8.32s\\
    \bottomrule
    \end{tabular}
    \caption{The comparison of the computational cost of different methods, given a $2920\times 4386$ input. \textit{N/A} in SAM~\cite{punnappurath2021spatially} means it is a parameter free method. \textit{Ours (serial)} means we substitute the commonly used PixelCNN based context model~\cite{cheng2020learned, minnen2018joint} for our proposed sRGB-guided context model. The arithmetic coding in our method can be further accelerated \cite{gpuar, chen2011accelerating, vsupol2005arithmetic} by running it on GPU.}
    \label{tab:cost}
\end{table}

\subsection{Reconstruction qualities with different bpp}
\label{sec:high_bpp}
We further explore the performance of the proposed model when we increase the bpp, \textit{i.e.,} by increasing the weight of the reconstruction term. We re-train a model with $\lambda=0.5$ instead of $0.05$ in the main paper. The results evaluated on JPEG images with the quality factor of $10$ are reported in Fig.  \ref{fig:bpp}. As shown in the figure, the performance of our method is greatly improved (around 6 in terms of PSNR) with the increase of the bpp while still remaining lower than Nam \textit{et al.} ~\cite{nam2022learning}.
Besides, we can significantly improve the reconstruction quality even if the file size of additionally saved metadata is almost negligible compared with the size of JPEG images. The visualizations of error maps are shown in Fig. \ref{fig:samsung} and Fig. \ref{fig:olym}. Some visualization results in the image space can be seen in Fig. \ref{fig:vis_image}. As we can see, our method achieves much better reconstruction quality with lower bpp than all other SOTA methods. In addition, due to the low quality of conditioned JPEG images, SAM~\cite{punnappurath2021spatially} fails in some of the blocks due to the non-exitance of solutions for the systems of linear equations.

\begin{table*}[htbp]
    \centering
    \begin{tabular}{c|cc|ccc}
    \toprule
    & \multicolumn{2}{c|}{\textbf{Fidelity}} & \multicolumn{3}{c}{\textbf{bpp}}\\
         & \multirow{2}{*}{PSNR} & \multirow{2}{*}{SSIM}  & Deterministic & Random sparse & The proposed\\
         & & & mask & mask  & learnable mask\\
    \midrule
    Samsung & 37.814 & 0.96757 & 3.102e-01 & 2.928e-01 & \textbf{2.854e-01}\\
    Olympus & 39.517 & 0.97745 & 2.967e-01 & 2.764e-01 & \textbf{2.694e-01}\\
    Sony & 39.936 & 0.97972 & 2.835e-01 &  2.691e-01 & \textbf{2.606e-01}\\
     \rowcolor[HTML]{EFEFEF} Mean & 39.089 & 0.97491 & 2.968e-01 & 2.794e-01 & \textbf{2.718e-01}\\
    \bottomrule
    \end{tabular}
    \caption{The ablation study on the proposed learnable order prediction model. We evaluate the performance of methods conditioned on JPEG images with quality factor of $10$ on NUS dataset.}
    \label{tab:mask}
\end{table*}

\subsection{Ablation study on learnable order masks}
 As illustrated in the main paper, our proposed sRGB-guided context model has two parts: the order prediction module and the iterative Gaussian entropy model. In this subsection, we explore the effectiveness of the design of the sampling masks during the compress/decompress processes. We evaluate the performance of the following strategies
\begin{itemize}
    \item A deterministic mapping formulated by
    \begin{equation}
        M_{i,j}^k = \left\{\begin{matrix}
        1, & \arg\max_{c} (\mathbf{m}_{i,j}^{c}) = k\\ 
        0, & \text{otherwise}
        \end{matrix}\right.
    \end{equation}
    \item Random sparse masks $\mathbf{M}^i$ that satisfy $\sum_{i=0}^N \mathbf{M}^i=\mathbf{1}$ where $\mathbf{1}$ is an all-one mask.
    \item The strategy adopted in the main paper. Specifically, we add a buffer to the model to save a pre-sampled random matrix $\mathbf{g}$ so that we can achieve the same sparse sampling masks during the compress/decompress process. Besides, the order masks are obtained with the guidance of sRGB images.
\end{itemize}

We evaluate the performance of the aforementioned strategies using the model illustrated in Sec.~\ref{sec:high_bpp}, \textit{i.e.}, the model trained with $\lambda=0.5$. 
The results are shown in Table~\ref{tab:mask}. Since the proposed sRGB-guided context model is a lossless compression model, all the competitors have exactly the same reconstruction quality. 
In terms of the bpp, the random sparse mask achieves better performance compared with the deterministic mask, due to the sparsity of sampling masks, i.e., the similarity between adjacent pixels can be better utilized. Our proposed learnable mask achieves the best performance which demonstrates the effectiveness of the proposed pre-sampling strategy and the introduced sRGB guidance.

\begin{figure*}[htbp]
    \centering
    \hspace{-0.4cm}
    \scalebox{0.86}{
    \subcaptionbox{Input\\(8 bit sRGB image)}{
    \includegraphics[height=0.56\linewidth, clip]{figure/appendix/bigfigure/input_o.jpg}
    }
    \hspace{-0.22cm}
    \subcaptionbox{InvISP~\cite{xing2021invertible}\\(bpp: N/A)}{
    \includegraphics[height=0.56\linewidth, trim=30 0 0 0,clip ]{figure/appendix/bigfigure/inv_o.jpg}}
    \hspace{-0.2cm}
    \subcaptionbox{SAM~\cite{punnappurath2021spatially} \\(bpp: 9.52e-3)}{
    \includegraphics[height=0.56\linewidth]{figure/appendix/bigfigure/wacv_o.jpg}}
    \hspace{-0.2cm}
    \subcaptionbox{Nam~\textit{et al.}\cite{nam2022learning} \\(bpp: 8.44e-1)}{
    \includegraphics[height=0.56\linewidth]{figure/appendix/bigfigure/cvpr_o.jpg}}
    \hspace{-0.2cm}
    \subcaptionbox{Ours\\(bpp: 0.2978)}{
    \includegraphics[height=0.56\linewidth]{figure/appendix/bigfigure/ours_o.jpg}}\hspace{0.cm}
    
    \includegraphics[height=0.56\linewidth, clip, trim=0 160 0 0]{figure/appendix/bigfigure/bar_0.05.pdf}\hspace{-0.1cm}
    
    \subcaptionbox{Raw image\\(After gamma correction)}{
    \includegraphics[height=0.56\linewidth]{figure/appendix/bigfigure/raw_o.jpg}}\hspace{-0.2cm
    }}

    \caption{
    Qualitative comparison results on the Olympus subset of NUS dataset~\cite{cheng2014illuminant}. We visualize the maximum value of the error among three channels on the pixel level. For better visualization, we apply gamma correction to the raw image to increase the visibility. 
    }
    \label{fig:olym}
\end{figure*}

\begin{figure*}[htbp]
    \centering
    \hspace{-0.4cm}
    \scalebox{0.86}{
    \subcaptionbox{Input\\(8 bit sRGB image)}{
    \includegraphics[height=0.625\linewidth, clip]{figure/appendix/bigfigure/input.jpg}
    }
    \hspace{-0.22cm}
    \subcaptionbox{InvISP~\cite{xing2021invertible}\\(bpp: N/A)}{
    \includegraphics[height=0.625\linewidth, trim=30 0 0 0,clip ]{figure/appendix/bigfigure/invisp.jpg}}
    \hspace{-0.2cm}
    \subcaptionbox{SAM~\cite{punnappurath2021spatially} \\(bpp: 9.52e-3)}{
    \includegraphics[height=0.625\linewidth]{figure/appendix/bigfigure/wacv.jpg}}
    \hspace{-0.2cm}
    \subcaptionbox{Nam~\textit{et al.}\cite{nam2022learning} \\(bpp: 8.44e-1)}{
    \includegraphics[height=0.625\linewidth]{figure/appendix/bigfigure/cvpr.jpg}}
    \hspace{-0.2cm}
    \subcaptionbox{Ours\\(bpp: 0.3141)}{
    \includegraphics[height=0.625\linewidth]{figure/appendix/bigfigure/ours.jpg}}\hspace{0.cm}
    
    \includegraphics[height=0.625\linewidth]{figure/appendix/bigfigure/bar_0.05.pdf}\hspace{-0.1cm}
    
    \subcaptionbox{Raw image\\(After gamma correction)}{
    \includegraphics[height=0.625\linewidth]{figure/appendix/big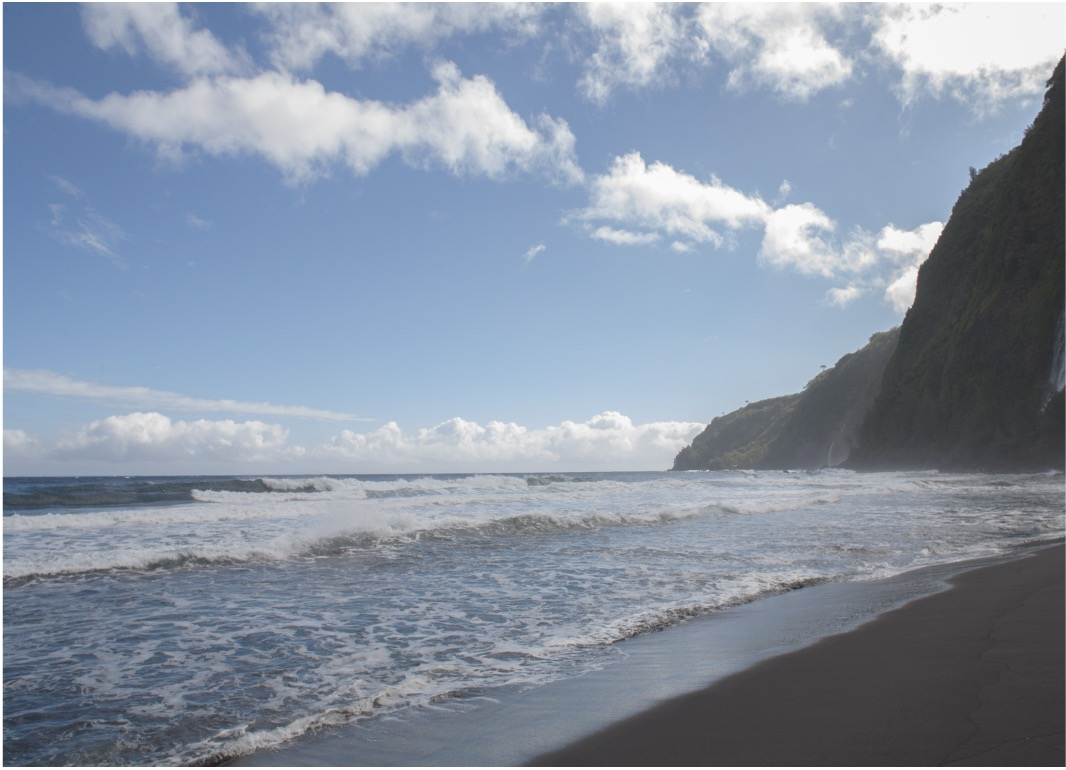}}\hspace{-0.2cm
    }}

    \caption{
    Qualitative comparison results on the Samsung subset of NUS dataset~\cite{cheng2014illuminant}. We visualize the maximum value of the error among three channels on the pixel level. For better visualization, we apply gamma correction to the raw image to increase the visibility. 
    }
    \label{fig:samsung}
\end{figure*}

\begin{figure}
    \centering
    \subcaptionbox{Input 8 bit JPEG images\\(quality factor 10)}{
    \includegraphics[height=1.18\linewidth]{figure/appendix/bigfigure/rgb_srgb.jpg}}\hspace{0.cm}
    \subcaptionbox{Nam \textit{et al.}~\cite{nam2022learning}\\(bpp: 0.844)}{
    \includegraphics[height=1.18\linewidth]{figure/appendix/bigfigure/rgb_cvpr.jpg}}\hspace{0.cm}
    \subcaptionbox{Ours\\(bpp: 0.269)}{
    \includegraphics[height=1.18\linewidth]{figure/appendix/bigfigure/rgb_ours.jpg}}\hspace{0.cm}
    \subcaptionbox{Raw image\\(After gamma correction)}{
    \includegraphics[height=1.18\linewidth]{figure/appendix/bigfigure/rgb_gt.jpg}}\hspace{0.cm}
    \caption{Qualitative comparison results on NUS dataset~\cite{cheng2014illuminant} in the image space. For better visualization, we apply gamma correction to raw/reconstructed raw images to increase the visibility.}
    \label{fig:vis_image}
\end{figure}
